# Supplementary material for: Spatially Constrained GAN for Face and Fashion Synthesis
Source: arXiv:1905.02320 source file (2021-12-06)
Supplement: Supplementary file 1 [file SCGAN_appendix.tex]

\subsection{Networks Architecture}
The detailed architecture of the generator, discriminator and segmentor networks in SCGAN are provided in Table \ref{tab_architect}. The shapes of the intermediate results are also provided. In summary, the generator takes a semantic segmentation, a latent vector and an attribute label as inputs step by step to synthesize a target image as described in Section \ref{section_generator}. The discriminator network has a discrimination output and a classification output which share same weights except the last layer. The segmentor network adopts a encoder-decoder architecture with a few residual blocks as bottle neck layers.

\small{
\begin{table*}[hbtp!]

\caption{Network architecture of SCGAN. (Abbrev: L=Layer; CONV=Convolutional layer; FC=Fully connected layer; RESBLK=Residual block; RESBLKUP=Residual block with upsampling; DECONV=Transposed convolutional layer; N=Number of neurons; K=Kernel Size; S=Stride; P=Padding; CONCAT=Concatenate; IN=Instance Normalization; RELU=Rectified Linear Unit; lRELU=leaky RELU; $n_z$=Dimension of latent vector; $n_c$=Number of attributes; $n_s$=Number of segmentation classes)}\label{tab_architect}

\centering
\begin{tabular}{|P{0.2cm}|p{6cm}|P{0.6cm} P{0.03cm} P{0.5cm} P{0.03cm} P{0.5cm}|}

  \hline
  \bf L	& \bf Generator & \multicolumn{5}{c|}{\bf Output Shape}\\
  \hline
  a	& \emph{Semantic segmentation} &$n_s$&$\times$&128&$\times$&128\\
  1	& CONV-(N64,K4,S2,P1),IN,RELU 	&64& $\times$&64&$\times$&64 \\
  2	& CONV-(N128,K4,S2,P1),IN,RELU 	&128& $\times$&32&$\times$&32 \\
  3	& CONV-(N256,K4,S2,P1),IN,RELU 	&256&$\times$&16&$\times$&16 \\
  4	& CONV-(N512,K4,S2,P1),IN,RELU 	&512&$\times$&8&$\times$&8 \\
  \hline
  b& \emph{Latent vector}	&$n_z$&$\times$&1&$\times$&1 \\
  b1& FC-(N8192),IN,RELU 	&64&$\times$&8&$\times$&8 \\
  \hline
  5	& CONCAT 4 with b1			&576&$\times$&8&$\times$&8 \\
  6	& RESBLKUP-(N64),IN,RELU 	&512&$\times$&16&$\times$&16 \\
  7	& RESBLKUP-(N64),IN,RELU 	&256&$\times$&32&$\times$&32 \\
  \hline
  c& \emph{Attribute label}	 	&$n_c$&$\times$&1&$\times$&1 \\
  c1& EXPAND			&$n_c$&$\times$&32&$\times$&32 \\
  \hline
  8	& CONCAT 7 with c1		&256+$n_c$&$\times$&32&$\times$&32 \\
  9	& RESBLKUP-(N64),IN,RELU 	&128&$\times$&64&$\times$&64 \\
  10& RESBLKUP-(N64),IN,RELU 	&64&$\times$&128&$\times$&128 \\
  11& CONV-(N3,K3,S1,P1),TANH		&3&$\times$&128&$\times$&128 \\
  \hline
  \bf L	& \bf Discriminator & \multicolumn{5}{c|}{\bf Output Shape}\\
  \hline
  a	& \emph{Input image}  		&3&$\times$&128&$\times$&128\\
  1	& CONV-(N64,K4,S2,P1),lRELU 	&64& $\times$&64&$\times$&64 \\
  2	& CONV-(N128,K4,S2,P1),lRELU 	&128& $\times$&32&$\times$&32 \\
  3	& CONV-(N256,K4,S2,P1),lRELU 	&256&$\times$&16&$\times$&16 \\
  4	& CONV-(N512,K4,S2,P1),lRELU 	&512&$\times$&8&$\times$&8 \\
  5	& CONV-(N1024,K4,S2,P),lRELU 	&1024&$\times$&4&$\times$&4 \\
  6	& CONV-(N2048,K4,S2,P1),lRELU 	&2048&$\times$&2&$\times$&2 \\
  \hline
  b& CONV-(N1,K3,S1,P1) 			&1&$\times$&2&$\times$&2 \\
  c& CONV-(N$n_c$,K3,S1,P1)  		&$n_c$&$\times$&1&$\times$&1 \\
  \hline
  \bf L	& \bf Segmentor & \multicolumn{5}{c|}{\bf Output Shape}\\
  \hline
  a	& \emph{Input image} 		&3&$\times$&128&$\times$&128\\
  1	& CONV-(N64,K4,S2,P1),IN,RELU 	&64& $\times$&64&$\times$&64 \\
  2	& CONV-(N128,K4,S2,P1),IN,RELU 	&128& $\times$&32&$\times$&32 \\
  \hline
  3	& RESBLK-(N128,K3,S1,P1),IN,RELU 	&128&$\times$&32&$\times$&32 \\
  4	& RESBLK-(N128,K3,S1,P1),IN,RELU 	&128&$\times$&32&$\times$&32 \\
  5	& RESBLK-(N128,K3,S1,P1),IN,RELU 	&128&$\times$&32&$\times$&32 \\
  6	& RESBLK-(N128,K3,S1,P1),IN,RELU 	&128&$\times$&32&$\times$&32 \\
  \hline
  7	& DECONV-(N64,K4,S2,P1),IN,RELU 	&64&$\times$&64&$\times$&64 \\
  8	& DECONV-(N32,K4,S2,P1),IN,RELU 	&32&$\times$&128&$\times$&128 \\
  9	& CONV-(N$n_s$,K3,S1,P1) 		&$n_s$&$\times$&128&$\times$&128 \\
  \hline
  
\end{tabular}
\end{table*}}
